# Supplementary material for: Infinitely Divisible Noise for Differential Privacy: Nearly Optimal Error in the High $\varepsilon$ Regime
Source: arXiv:2504.05202 source file (2025-04-07)
Supplement: Supplementary file 1 [file multiscale-general.tex]

\subsection{The abstract multi-scale mechanism}
\todo{figure out the best way to do this. Start abstract or just generalize after the MSDLap mechanism?}
We define the \emph{$(\mathcal{D}, \eps, \Delta)$-multi-scale mechanism mechanism} with parameters $\eps > 0, \Delta \in \N$, and $\mathcal{D}$ an infinitely divisible discrete probability distribution
for function $q$ works as follows:
\begin{itemize}
\item Sample $X_1, \dots, X_{\Delta} \sim \mathcal{D}$.
\item Output $q(X) + \sum_{i=1}^{\Delta} i \cdot X_i$.
\end{itemize}

Note that it is obvious that $\sum_{i=1}^{\Delta} i \cdot X_i$ is infinitely divisible, since each $X_i$ is infinitely divisible. We give a proof below that if $\mathcal{D}$ satisfies $\eps$-DP for $\Delta = 1$ queries, this mechanism is $\eps$-DP.

\begin{theorem} \label{thm:multi-scale-dlap}
For any $q, q': X^d \to \Z$ where $\Delta(q') = 1$, the $(\mathcal{D}, \eps, \Delta = \Delta(q))$-multi-scale mechanism is $\eps$-DP if the mechanism $q'(X) + \mathcal{D}$ is $\eps$-DP. Furthermore, for $\eps \geq 1$, the MSE is $O(\Delta^3 \Var[\mathcal{D}])$.
\end{theorem}

\begin{proof}
\emph{(Privacy)} Consider any two neighboring datasets $x, x'$. We will show that $\eps \geq \dr{q(x) + \sum_{i=1}^{\Delta} X_i}{q(x') + \sum_{i=1}^{\Delta} X_i} = \dr{q(x) - q(x') + \sum_{i=1}^{\Delta} X_i}{\sum_{i=1}^{\Delta} X_i}$. If $q(x) = q(x')$, then this is obvious. Otherwise, let $i^* = |q(x) - q(x')|$. From \Cref{lem:post-processing}, we have
\begin{align*}
&\dr{q(x) - q(x') + \sum_{i=1}^{\Delta} X_i}{\sum_{i=1}^{\Delta} X_i} \\
&\leq \dr{q(x) - q(x') + i^* \cdot X_i}{i^* \cdot X_i} \\
&= \dr{1 + X_i}{X_i} \\
&\leq \eps,
\end{align*}
where the last inequality follows from $X_i \sim \mathcal{D}$ and the privacy assumption on $\mathcal{D}$.

\emph{(Accuracy)} The MSE of the mechanism is
\begin{align*}
\Var\left(\sum_{i=1}^{\Delta} i \cdot X_i\right) &= \sum_{i=1}^{\Delta} \Var[i \cdot X_i]\\
&= \frac{1}{6}\Delta(\Delta + 1)(2\Delta + 1) \Var[\mathcal{D}] \\
&= O(\Delta^3 \cdot \Var[\mathcal{D}]). & \qedhere
\end{align*}
\end{proof}

\begin{corollary}
    The $(\DLap(\eps), \eps, \Delta)$-multi-scale mechanism satisfies $\eps$-DP and the MSE is $O(\Delta^3 e^{-\eps})$.
\end{corollary}
\begin{proof}
This follows directly from the fact that 
$$
\Var[\DLap(\eps)] = \frac{1}{\cosh(\eps) - 1} = O(e^{-\eps}). \qedhere
$$
\end{proof}

\begin{corollary}
    The $(\GDL(\beta, a), \eps, \Delta)$-multi-scale mechanism satisfies $\max(a, a - \log \beta)$-DP and the MSE is $O\left(\Delta^3 \beta e^{-\eps}\right)$. Furthermore, the mechanism is closed under summation.
\end{corollary}
\begin{proof}
The privacy follows from \Cref{thm:main-epsilon} and \Cref{cor:hyper-ratio}. The accuracy follows as $\Var[\GDL(a, \beta)] = \frac{\beta}{\cosh(a)-1} = O(\beta e^{-\eps})$. The mechanism is closed under summation, as every individual $\GDL$ random variable in the multi-scale sum is closed under summation.
\end{proof}

\begin{corollary}
    For a fixed $\Delta$ and arbitrarily large $\eps$, the MSE of the $(\DLap(\eps), \eps, \Delta)$-multi-scale mechanism matches (including constants) the discrete staircase mechanism with $r=1$ of $\frac{1}{3}e^{-\eps} \Delta (\Delta + 1)(2\Delta + 1)$
\end{corollary}
\begin{proof}
    The variance of the discrete staircase distribution with $r=1$ is shown in \Cref{obs:dstair-var-large}. We will show the DLap-MSM matches it by taking the limit:

\begin{align*}
\lim_{\eps\to\infty} e^\eps \Var\left(\sum_{i=1}^{\Delta} i \cdot X_i\right) 
&= \lim_{\eps\to\infty} e^\eps \frac{\Delta(\Delta + 1)(2\Delta + 1)}{6 (\cosh(\eps) - 1)}\\
&= \frac{1}{6}\Delta(\Delta + 1)(2\Delta + 1) \cdot \lim_{\eps\to\infty}  \frac{e^\eps}{\cosh(\eps)-1} \\
&= \frac{1}{3}\Delta(\Delta + 1)(2\Delta + 1)
\end{align*}
\end{proof}

\subsubsection{The multi-scale multi-parameter mechanism}

We generalize the multi-scale mechanism to help us match the error in~\cite{geng2014optimal} for every setting of parameters $\Delta, \eps$. The \emph{$(\mathcal{D}, \mathcal{D}_r, \eps, \Delta)$-multi-scale mechanism} with parameters $\eps > 0, \Delta \in \mathbb{N}$, and $\mathcal{D}, \mathcal{D}_r$ infinitely divisible discrete probability distributions for a function $q$ works as follows:

\begin{itemize}
\item Let $\Delta_0 = \lfloor \Delta / r \rfloor$
\item Sample $X_1, X_2 \dots, X_{\Delta_0} \sim \mathcal{D}$ and $X^* \sim \mathcal{D}_{r}$.
\item Output $q(X) + X^* + \sum_{i=1}^{\Delta_0} r \cdot i \cdot X_i$.
\end{itemize}

We state the theorem below where $r \in \{0, \dots, \Delta\}$ is the free parameter so that it matches the ``$r$'' parameter in the discrete staircase mechanism as presented in \cite{geng2014optimal}.

\begin{theorem} \label{thm:multi-scale-multi-param}
For any $q, q', q'': X^d \to \Z$ where $\Delta(q) = 1, \Delta(q') = 1, \Delta(q'') = r$, the $(\mathcal{D}, \mathcal{D}_r, \eps, \Delta = \Delta(q))$-multi-scale mechanism is $\eps$-DP if the mechanism $q'(X) + \mathcal{D}$ is $\eps -1 $-DP, and the mechanism $q''(X) + \mathcal{D}_r$ is $1$-DP. Furthermore, for $\eps \geq 1$, the MSE is $O(\Var[\mathcal{D}_r] + \frac{\Delta^3 \Var[\mathcal{D}]}{r+1})$.
\end{theorem}
\begin{proof}

\todo{finish?}

First, note that if $r = 0$, then the claimed bound follows from \Cref{thm:multi-scale-dlap}. Thus, we can henceforth assume that $r \geq 1$.

Note that it is obvious that $Z := X^* + \sum_{i=1}^{\Delta_0} r \cdot i \cdot X_i$ is infinitely divisible, since each $X_i$ and $X^*$ are infinitely divisible.

\emph{(Privacy)} 
For notational convenience, we assume that we also have $X_0 \sim \DLap(\eps - 1)$. 
Consider any two neighboring datasets $x, x'$. We assume w.l.o.g. that $q(x) \geq q(x')$. We will show that $\eps \geq \dr{q(x) + Z}{q(x') + Z} = \dr{q(x) - q(x') + Z}{Z}$. 
Let $i^* = \lfloor (q(x) - q(x')) / r\rfloor$ and $j^* = q(x) - q(x') - r \cdot i^*$. Note that $i^* \in \{0, \dots, \Delta_0\}$ and $j^* \in \{0, \dots, r\}$. From \Cref{lem:post-processing}, \Cref{lem:tri-ineq},  then \Cref{lem:post-processing} again, we have
\begin{align*}
&\dr{q(x) - q(x') + Z}{Z} \\
&\leq \dr{q(x) - q(x') + r \cdot i^* \cdot X_i + X^*}{r \cdot i^* \cdot X_i + X^*} \\
&= \dr{r \cdot i^* + j^* + r \cdot i^* \cdot X_i + X^*}{r \cdot i^* \cdot X_i + X^*} \\
&\leq \dr{r \cdot i^* + j^* + r \cdot i^* \cdot X_i + X^*}{r \cdot i^* + r \cdot i^* \cdot X_i + X^*} \\ 
&\hphantom{abc} + \dr{r \cdot i^* + r \cdot i^* \cdot X_i + X^*}{r \cdot i^* \cdot X_i + X^*} \\
&=  \dr{j^* + r \cdot i^* \cdot X_i + X^*}{r \cdot i^* \cdot X_i + X^*} \\
&\hphantom{abc} + \dr{r \cdot i^* + r \cdot i^* \cdot X_i + X^*}{r \cdot i^* \cdot X_i + X^*} \\
&\leq  \dr{j* + X^*}{X^*} + \dr{1 + X_i}{X_i} \\
&\leq 1 + (\eps - 1) = \eps,
\end{align*}
where the last inequality follows from $X_{i^*} \sim \DLap(\eps - 1)$ and $X^* \sim \DLap(1/r)$.

\emph{(Accuracy)} The MSE of the mechanism is
\begin{align*}
&\Var\left(X^* + \sum_{i=1}^{\Delta_0} r \cdot i \cdot X_i\right) 
= \Var(X^*) + \sum_{i=1}^{\Delta_0} \Var(r \cdot i \cdot X_i) \\
&= O(r^2) +  \sum_{i=1}^{\Delta_0} r^2 i^2 \cdot \Var(X_i) \\
&= 
O(r^2) + r^2 \cdot \frac{\Delta_0(\Delta_0 + 1)(2\Delta_0 + 1)}{6 (\cosh(\eps - 1) - 1)} \\
&= O(r^2 + e^{-\eps} \Delta^3 / r) & \qedhere
\end{align*}
\end{proof}

It should be noted that, by plugging in $r = 0, r = \lceil e^{-\eps/3} \Delta \rceil$, we get the following corollary:
\begin{corollary}
For any $\eps \geq 2$ and every $r \in \{0, \dots, \Delta\}$, there exists an infinitely divisible discrete noise-addition mechanism that is $\eps$-DP for any $q: X^d \to \Z$ with $\Delta(q) \leq \Delta$ with MSE $O(\Delta^2 \min\{e^{-\eps} \Delta, e^{-2\eps/3}\})$. 
\end{corollary}
